# Supplementary material for: PartGlot: Learning Shape Part Segmentation from Language Reference Games
Source: arXiv:2112.06390 source file (2022-03-30)
Supplement: Supplementary file 2 [file image_list.tex]

\Image{figures/\suppSegDir/chair_00.png}
\Image{figures/\suppSegDir/chair_01.png}
\Image{figures/\suppSegDir/chair_02.png}
\Image{figures/\suppSegDir/chair_03.png}
\Image{figures/\suppSegDir/chair_04.png}
\Image{figures/\suppSegDir/chair_05.png}
\Image{figures/\suppSegDir/chair_06.png}
\Image{figures/\suppSegDir/chair_07.png}
\Image{figures/\suppSegDir/chair_08.png}
\Image{figures/\suppSegDir/chair_09.png}
\Image{figures/\suppSegDir/chair_10.png}

\Image{figures/\suppSegDir/chair_25.png}
\Image{figures/\suppSegDir/chair_26.png}
\Image{figures/\suppSegDir/chair_27.png}
\Image{figures/\suppSegDir/chair_28.png}
\Image{figures/\suppSegDir/chair_29.png}
\Image{figures/\suppSegDir/chair_30.png}
\Image{figures/\suppSegDir/chair_31.png}
\Image{figures/\suppSegDir/chair_32.png}
\Image{figures/\suppSegDir/chair_33.png}
\Image{figures/\suppSegDir/chair_34.png}
\Image{figures/\suppSegDir/chair_35.png}
\Image{figures/\suppSegDir/chair_36.png}
\Image{figures/\suppSegDir/chair_37.png}
\Image{figures/\suppSegDir/chair_38.png}

\Image{figures/\suppSegDir/table_00.png}
\Image{figures/\suppSegDir/table_01.png}
\Image{figures/\suppSegDir/table_02.png}
\Image{figures/\suppSegDir/table_03.png}
\Image{figures/\suppSegDir/table_04.png}
\Image{figures/\suppSegDir/table_05.png}
\Image{figures/\suppSegDir/table_06.png}
\Image{figures/\suppSegDir/table_07.png}
\Image{figures/\suppSegDir/table_08.png}
\Image{figures/\suppSegDir/table_09.png}
\Image{figures/\suppSegDir/table_10.png}
\Image{figures/\suppSegDir/table_11.png}
\Image{figures/\suppSegDir/table_12.png}
\Image{figures/\suppSegDir/table_13.png}
\Image{figures/\suppSegDir/table_14.png}
\Image{figures/\suppSegDir/table_15.png}
\Image{figures/\suppSegDir/table_16.png}
\Image{figures/\suppSegDir/table_17.png}
\Image{figures/\suppSegDir/table_18.png}
\Image{figures/\suppSegDir/table_19.png}
\Image{figures/\suppSegDir/table_20.png}
\Image{figures/\suppSegDir/table_21.png}
\Image{figures/\suppSegDir/table_22.png}
\Image{figures/\suppSegDir/table_23.png}
\Image{figures/\suppSegDir/table_24.png}
\Image{figures/\suppSegDir/table_25.png}
\Image{figures/\suppSegDir/table_26.png}
\Image{figures/\suppSegDir/table_27.png}
\Image{figures/\suppSegDir/table_28.png}
\Image{figures/\suppSegDir/table_29.png}
\Image{figures/\suppSegDir/table_30.png}
\Image{figures/\suppSegDir/table_31.png}
\Image{figures/\suppSegDir/table_32.png}
\Image{figures/\suppSegDir/table_33.png}
\Image{figures/\suppSegDir/table_34.png}
\Image{figures/\suppSegDir/table_35.png}
\Image{figures/\suppSegDir/table_36.png}
\Image{figures/\suppSegDir/table_37.png}
\Image{figures/\suppSegDir/table_38.png}

\Image{figures/\suppSegDir/lamp_02.png}
\Image{figures/\suppSegDir/lamp_03.png}
\Image{figures/\suppSegDir/lamp_04.png}
\Image{figures/\suppSegDir/lamp_05.png}
\Image{figures/\suppSegDir/lamp_06.png}
\Image{figures/\suppSegDir/lamp_07.png}
\Image{figures/\suppSegDir/lamp_08.png}
\Image{figures/\suppSegDir/lamp_09.png}
\Image{figures/\suppSegDir/lamp_10.png}
\Image{figures/\suppSegDir/lamp_11.png}
\Image{figures/\suppSegDir/lamp_12.png}
\Image{figures/\suppSegDir/lamp_13.png}
\Image{figures/\suppSegDir/lamp_14.png}
\Image{figures/\suppSegDir/lamp_15.png}
\Image{figures/\suppSegDir/lamp_16.png}
\Image{figures/\suppSegDir/lamp_17.png}
\Image{figures/\suppSegDir/lamp_18.png}
\Image{figures/\suppSegDir/lamp_19.png}
\Image{figures/\suppSegDir/lamp_20.png}
\Image{figures/\suppSegDir/lamp_21.png}
\Image{figures/\suppSegDir/lamp_22.png}
\Image{figures/\suppSegDir/lamp_23.png}
\Image{figures/\suppSegDir/lamp_24.png}
\Image{figures/\suppSegDir/lamp_25.png}
\Image{figures/\suppSegDir/lamp_26.png}
\Image{figures/\suppSegDir/lamp_27.png}
\Image{figures/\suppSegDir/lamp_28.png}
\Image{figures/\suppSegDir/lamp_29.png}
\Image{figures/\suppSegDir/lamp_30.png}
\Image{figures/\suppSegDir/lamp_31.png}
\Image{figures/\suppSegDir/lamp_32.png}
\Image{figures/\suppSegDir/lamp_33.png}
\Image{figures/\suppSegDir/lamp_34.png}
\Image{figures/\suppSegDir/lamp_35.png}
\Image{figures/\suppSegDir/lamp_36.png}

\Image{figures/\suppSegDir/airplane_00.png}
\Image{figures/\suppSegDir/airplane_01.png}
\Image{figures/\suppSegDir/airplane_02.png}
\Image{figures/\suppSegDir/airplane_03.png}
\Image{figures/\suppSegDir/airplane_04.png}
\Image{figures/\suppSegDir/airplane_05.png}
\Image{figures/\suppSegDir/airplane_06.png}
\Image{figures/\suppSegDir/airplane_07.png}
\Image{figures/\suppSegDir/airplane_08.png}
\Image{figures/\suppSegDir/airplane_09.png}
\Image{figures/\suppSegDir/airplane_10.png}
\Image{figures/\suppSegDir/airplane_11.png}
\Image{figures/\suppSegDir/airplane_12.png}
\Image{figures/\suppSegDir/airplane_13.png}
\Image{figures/\suppSegDir/airplane_14.png}
\Image{figures/\suppSegDir/airplane_15.png}
\Image{figures/\suppSegDir/airplane_16.png}
\Image{figures/\suppSegDir/airplane_17.png}
\Image{figures/\suppSegDir/airplane_18.png}
\Image{figures/\suppSegDir/airplane_19.png}
\Image{figures/\suppSegDir/airplane_20.png}
\Image{figures/\suppSegDir/airplane_21.png}
\Image{figures/\suppSegDir/airplane_22.png}
\Image{figures/\suppSegDir/airplane_23.png}
\Image{figures/\suppSegDir/airplane_24.png}
\Image{figures/\suppSegDir/airplane_25.png}
\Image{figures/\suppSegDir/airplane_26.png}
\Image{figures/\suppSegDir/airplane_27.png}
\Image{figures/\suppSegDir/airplane_28.png}
\Image{figures/\suppSegDir/airplane_29.png}
\Image{figures/\suppSegDir/airplane_30.png}
\Image{figures/\suppSegDir/airplane_31.png}
\Image{figures/\suppSegDir/airplane_32.png}
\Image{figures/\suppSegDir/airplane_33.png}
\Image{figures/\suppSegDir/airplane_34.png}
\Image{figures/\suppSegDir/airplane_35.png}
\Image{figures/\suppSegDir/airplane_36.png}
\Image{figures/\suppSegDir/airplane_37.png}

\Image{figures/\suppSegDir/car_00.png}
\Image{figures/\suppSegDir/car_01.png}
\Image{figures/\suppSegDir/car_02.png}
\Image{figures/\suppSegDir/car_03.png}
\Image{figures/\suppSegDir/car_04.png}
\Image{figures/\suppSegDir/car_05.png}
\Image{figures/\suppSegDir/car_06.png}
\Image{figures/\suppSegDir/car_07.png}
\Image{figures/\suppSegDir/car_08.png}
\Image{figures/\suppSegDir/car_09.png}
\Image{figures/\suppSegDir/car_10.png}
\Image{figures/\suppSegDir/car_11.png}
\Image{figures/\suppSegDir/car_12.png}
\Image{figures/\suppSegDir/car_13.png}
\Image{figures/\suppSegDir/car_14.png}
\Image{figures/\suppSegDir/car_15.png}
\Image{figures/\suppSegDir/car_16.png}
\Image{figures/\suppSegDir/car_17.png}
\Image{figures/\suppSegDir/car_18.png}
\Image{figures/\suppSegDir/car_19.png}
\Image{figures/\suppSegDir/car_20.png}
\Image{figures/\suppSegDir/car_21.png}
\Image{figures/\suppSegDir/car_22.png}
\Image{figures/\suppSegDir/car_23.png}
\Image{figures/\suppSegDir/car_24.png}
\Image{figures/\suppSegDir/car_25.png}
\Image{figures/\suppSegDir/car_26.png}
% \Image{figures/\suppSegDir/car_27.png}
\Image{figures/\suppSegDir/car_28.png}
